# Supplementary material for: Improving the convergence of SGD through adaptive batch sizes
Source: arXiv:1910.08222 source file (2023-09-27)
Supplement: Supplementary file 1 [file appendix-tune-padadamp.tex]

% Base tuning: launch 1000 jobs random searches. 100 epochs.
%   Submission: run.py
%   Viz: exp-fashion-mnist/Viz-tuning3-1000.ipynb
%   Data: _data/cluster-2020-04-03.zip
%
% Second round: take top 200 jobs. Average 4. 100 epochs. Minimum: final loss,
% with minimum model updates in min + 0.005.
%   Submission: run2.py
%   Viz: exp-fashion-mnist/Viz-tuning4.ipynb
%   Data: _data/cluster-2020-04-14-recovery.zip
%
% Third round:
%   Submission: run3.py
%   Viz: Viz-final.ipynb
%   Data: _data/cluster-2020-05-01.zip

Fashion MNIST is a dataset with 60,000 training examples and 10,000 testing
examples. Each example includes a $28\times 28$ image that falls in one of 10
classes (e.g., ``coat'' or ``bag'')~\cite{fmnist}. The standard pre-processing
in PyTorch's MNIST example is used.\footnote{The transform at
\href{https://github.com/pytorch/examples/blob/b9f3b2ebb9464959bdbf0c3ac77124a704954828/mnist/main.py\#L105}{\texttt{http://github.com/pytorch/examples/\ldots/mnist/main.py\#L105}}
is used; the resulting pixels value have a mean of 0.504 and a standard
deviation of 1.14, not zero mean and unit variance as is typical for
preprocessing. The model used has about 110 thousand parameters and includes
biases in all layers, likely resolving any issues.}

The CNN used has about 111,000 parameters that specify 3 convolutional layers
with max-pooling and 2 fully-connected layers, with ReLU activations after
every layer.  This CNN is small enough to evaluate \AdaDamp's batch size,
especially since the batch size is only evaluated once every $d=50$ model
updates.

The hyperparameter optimization process for followed this data flow. For each
optimizer, the following steps were performed:

\begin{enumerate}

    \item Randomly sample about 1000 hyper-parameters from the spaces defined
        in Section~\ref{sec:exp-fmnist-space}.  Train these models for 100
        epochs.\footnote{All jobs did not complete in time. AdaDamp completed
        802 jobs and all other optimizers completed between 945 and 963 jobs.}
        Use 20\% of the train dataset for validation and 80\% for training.

        \item Select 200 of the best performing hyperparameters from the
            previous step as measured against validation loss. Report the
            average performance over 5 different validation sets after training
            for 100 epochs.

        \item Select the hyperparameters that had validation loss within 0.005
            of the minimum and the minimum number of model updates.

        \item With these parameters, train the model for 150 epochs on the
            entire training set and evaluate performance on the testing set.

\end{enumerate}

Step 2 is somewhat similar to median elimination~\cite[Section
3.2.2]{golovin2017google}. We performed step 3 because model updates are also a
metric shown in the Figure~\ref{fig:exp-fashion-mnist}, and there were 54 such
models for Adagrad, 6 for SGD and 26 for GeoDamp.

There were 8 such models for \AdaDamp. However, between step 3 and before step 4
additional modification were to these hyperparameter to encourage better
performance and to slightly modify the implementation. For all tuned
optimizers, we evaluated performance on the testing once. We did this by
measuring 200 different random seeds.

\subsubsection{Hyperparameter sampling space and tuned values}\label{sec:exp-fmnist-space}%
%base:
%  dataset: [fashionmnist]
%  lr: {"space": "log", "base": 10, "low": -2.0, "high": -0.0}
%adagrad:  # 4 discrete x 1cnts = 16 (4 per cnts)
%  initial_batch_size: [32, 64, 128, 256]
%  lr: {"space": "log", "base": 10, "low": -2.5, "high": -1.5}
%adadamp:  # 8 x 6 x 9 x 2cnts = 432 x 2cnts = 3,546
%  initial_batch_size: [10, 12, 14, 16, 24, 32, 48, 64]
%  max_batch_size: [64, 128, 256, 512, 1024, 2048]
%  dwell: [5, 10, 20, 50, 100, 200, 500, 1000, 2000]
%  approx_loss: [true]
%padadamp:  # 8 x 6 x 9 x 2cnts x 3cnts = 432 x 6cnts = 10,368
%  initial_batch_size: [10, 12, 14, 16, 24, 32, 48, 64]
%  max_batch_size: [64, 128, 256, 512, 1024, 2048]
%  dwell: [5, 10, 20, 50, 100, 200, 500, 1000, 2000]
%  batch_growth_rate: {"space": "log", "base": 10, "low": -3.0, "high": 0.0}
%geodamp:  # 5 x 9 x 3 x 4 x 2cnts = 540 x 2cnts = 4,320
%  dampingdelay: [4, 6, 8, 12, 16]
%  dampingfactor: [3, 4, 5, 6, 7, 8, 9, 10, 11]
%  initial_batch_size: [16, 32, 64]
%  max_batch_size: [512, 1024, 2048, 4096]
%geodamplr:  # 5 x 8 x 4 x 2cnts = 160 x 2cnts = 1,280
%  dampingdelay: [4, 8, 10, 12, 16]
%  dampingfactor: [1.4, 1.7, 2, 3, 4, 5, 6, 7]
%  initial_batch_size: [32, 64, 128, 256]

The learning rates are sampled log-uniformly at random between the two values
supplied below. All other choices are made uniformly at random from the
supplied list.

\begin{itemize}
    \item \textbf{Adagrad}:
        \begin{itemize}
            \item Learning rate: between $10^{-2.5}$ and $10^{-1.5}$ \textbf{(tuned value: $10^{-2.249}$)}.
            \item Batch size: [32, 64, 128, 256] \textbf{(tuned value: 256)}.
        \end{itemize}
    \item \textbf{\AdaDamp}:
        \begin{itemize}
            \item Learning rate: between $10^{-2}$ and $10^{0}$ \textbf{(tuned value: $10^{-1.329}$)}.
            \item Initial batch size: [10, 12, 14, 16, 24, 32, 48, 64] \textbf{(tuned value: 64)}.
            \item Relaxation time: [5, 10, 20, 50, 100, 200, 500, 1000, 2000] \textbf{(tuned value: 50)}.
            \item Maximum batch size: [64, 128, 256, 512, 1024, 2048] \textbf{(tuned value: 1024)}.
        \end{itemize}
    \item \textbf{GeoDamp}:
        \begin{itemize}
            \item Learning rate: between $10^{-2}$ and $10^{0}$ \textbf{(tuned value: $10^{-1.304}$)}.
            \item Initial batch size: [16, 32, 64] \textbf{(tuned value: 32)}.
            \item Damping delay (epochs): [4, 6, 8, 12, 16] \textbf{(tuned value: 6)}.
            \item Damping factor: [3, 4, 5, 6, 7, 8, 9, 10, 11] \textbf{(tuned value: 5)}.
            \item Maximum batch size: [512, 1024, 2048, 4096] \textbf{(tuned value: 4096)}.
        \end{itemize}
    \item \textbf{SGD}:
        \begin{itemize}
            \item Learning rate: between $10^{-2}$ and $10^{0}$ \textbf{(tuned value: $10^{-1.760}$)}.
            \item  Damping delay (epochs): [4, 8, 10, 12, 16] \textbf{(tuned value: 16)}.
            \item  Damping factor: [1.4, 1.7, 2, 3, 4, 5, 6, 7] \textbf{(tuned value: 2)}.
            \item  Batch size: [32, 64, 128, 256] \textbf{(tuned value: 256)}.
        \end{itemize}
\end{itemize}

If the damping factor is $d$ and the damping delay is $e$ epochs, the batch
size increases by a factor of $d$ or the step size decays by a factor of $d$
every $e$ epochs.

\subsection{Forest cover types}\label{app:padadamp}

\subsubsection{Dataset}

The dataset used is the UCI forest cover types
dataset~\cite{blackard1999comparative}. This dataset includes a total of
581,012 examples of forests that are in ``four wilderness areas located in the
Roosevelt National Forest of northern Colorado. These areas represent forests
with minimal human-caused disturbances, so that existing forest cover types are
more a result of ecological processes rather than forest management
practices.''

Each example has 54 integer features. Some examples of features names are
include elevation, slope, soil type, and horizontal distance to fire points.
Each examples also includes information on the classification, the ``cover type'' or the dominant vegetation growing in the image.

For each of the continuous features, we process by subtracting the mean and
making each feature have unit variance. There are 10 features like this, and
the other features are 0/1 indicator variables encoding soil type (40 columns)
and wilderness area type (4 columns).

This dataset is projected into a polynomial features space with degree $d=2$.
In this, only interactions between variables are considered (so for features
$x$ and $y$, only $xy$ is considered and not $x^2$ or $y^2$) and columns with
one unique value are filtered out (which is important for the indicator
columns). In total, there are 613 features.

\subsubsection{Model}

A linear model is trained on the convex categorical cross entropy loss for the
7 forest types. This linear model had a bias term for each of the 7 outputs.

\subsubsection{Hyperparameters}\label{app:pada-params}

All optimizers have the same initialization and data ordering.
These hyperparameters are common for:

\begin{itemize}
        \tightlist
    \item Learning rate: $\bm{0.9\cdot 10^{-3}}$
    \item Weight decay: $\bm{10^{-6}}$
    \item Momentum: $\bm{0.9}$.\footnote{Not used for ASGD.} This momentum is used
        with PyTorch's implementation of Nesterov momentum by~\citet{sutskever2013importance}.
    \item Initial batch size: $\bm{256}$.
\end{itemize}

In addition, here are some optimizer specific hyperparameters:

\begin{itemize}
        \tightlist

    \item \PadaDamp~batch size growth rate and SGD's learning rate decay rate:
        rate of $\bm{0.0819239}$.

    \item \PadaDamp~and SGD's dwell: $5$ model updates. However, the batch size
        growth rate changes the batch size by 1 every about every 12 model
        updates, so the dwell hyperparameter is irrelevant for \PadaDamp.

    \item \PadaDamp's maximum batch size: $\bm{2048}$, which only applies to \PadaDamp.

    \item ASGD starts averaging after $\bm{10^3}$ \textbf{model updates}.

    \item GeoDamp maximum batch size: \textbf{4096}.

    \item GeoDamp damping factor: $\approx \bm{6.605}$.
    \item GeoDamp damping delay: $\bm{200}$ \textbf{epochs}.

\end{itemize}

\subsubsection{Hyperparameter optimization}
\label{app:padadamp-hyperopt}

The Hyperband implementation in Dask-ML~\cite{sievert2019better} was used to
tune this model/dataset. We use the validation loss as the metric when
deciding to stop models. For both optimizers, we sample 49 hyperparameters and
initialize models with those hyperparameters.

\begin{itemize}
        \tightlist

    \item Initial batch size: $[2^5, 2^6, \ldots, 2^9]$.

    \item Maximum batch size: $[2^6, 2^7, \ldots, 2^{10}]$.

    \item Learning rate: chosen in a log-uniform fashion\footnote{``Chosen in a
        log-uniform fashion between $10^a$ and $10^b$'' means that $x$ is
        chosen uniformly between $a$ and $b$ and a value of $10^x$ is
        produced.} between $0.5\cdot 10^{-4}$ and $10^{-1}$.

    \item Momentum: chosen uniformly between 0 and 1.

    \item \PadaDamp~and SGD's learning decay rate: chosen in a log-uniform
        fashion between values of $10^{-3}$ and $10^{-1}$.

    \item \PadaDamp~and SGD's dwell: selected uniformly from the list $[1, 2,
        5, 10, 20, 50, 100, 200]$.

    \item GeoDamp maximum batch size: randomly chosen from $[1024, 2048, 4096,
        8192]$.

    \item GeoDamp ``damping delay'' (epoch), the number of epochs to wait
        before the batch size increases. Chosen randomly from the list
        $[50, 100, 200, 500, 2000]$.

    \item GeoDamp ``damping factor,'' the multiplicative factor the batch size
        increases/learning rate decays by. Chosen in a log-uniform fashion
        between values of 1 and 10.

\end{itemize}

The validation set consisted of 20\% of the examples training dataset, or
40,000 examples. From this, hyperparameters were found for all optimizers with
Hyperband and representative values were chosen from the best values. These
representative values are used in Appendix~\ref{app:pada-params}.

\subsubsection{HSGD comparison}\label{app:cnvx-hsgd}

We modify HSGD~\cite{zhou2018new} in two ways to incorporate maximum
batch size.
Specifically, ``HSGD-1'' and ``HSGD-2'' decay the learning rate like
$\bigO{1/k}$ and $\bigO{1/k^2}$ respectively after the maximum batch size is
reached.
Since HSGD requires that only pass of the data be completed, our
implementation shuffles the data once per epoch and samples each point once per
epoch. This works in practice though it does not fit in their mathematical
framework.

HSGD-1 relies on the classic SGD analysis by \citet{robbins1951}, which
requires that the step size $\gamma_k$ satisfy $\sum_{i=1}^\infty \gamma_k =
\infty$ and $\sum_{i=1}^\infty \gamma_k^2 < \infty$. Clear, having $\gamma_k =
\sfrac{k_{\max}}{k_{\max} + k}$ if the maximum batch size is reached at
$k_{\max}$ satisfies those conditions.  The differences between HSGD-1 and
\PadaDamp~are marginal and very likely come down to implementation
details:\footnote{Specifically, the learning rate in \PadaDamp~decays like
$\gamma_k = \gamma_0 B_{\max} / (m\cdot k)$ for some rate $m$, and the learning
rate for HSGD-1 decays like $\gamma_k = \gamma_0 k_{\max}/(k_{\max} + m(k -
k_{\max}))$ where $k_{\max}$ is the model update when maximum batch size is
reached.} both HSGD-1 and \PadaDamp~decay the learning rate like $\bigO{1/k}$
after the maximum batch size is reached in
Figure~\ref{fig:padadamp-hsgd-batch-size}.

HSGD-2 has a less formal justification, one that's related to simulated
annealing. Increasing the batch size or decreasing the learning rate
can be thought of reducing the ``noise scale'' or variance of the model
update~\cite{smith2017b}. The variance of the model updates is given by
$\sigma_U^2$ and
$$\Align{
    \sigma_U^2 = \var\left(\frac{\gamma_k}{B_k}\sum_{i=1}^{B_k} \grad f_{i_s} (\wb_k)\right)
    =\frac{\gamma_k\sigma_f^2}{B_k}
}$$
A variance of $\alpha \cdot\sigma_U^2$ can be obtained by either decreasing the
learning rate $\gamma_k$ by a factor of $\alpha$ or increasing the batch size
$B_k$ by a factor of $\alpha$.

HSGD-1 differs from simulated annealing, which does not have any rate changes
in the temperature decay schedules~\cite{nourani1998}. Notably, the temperature
decay schedules in \citet{nourani1998} are linear, exponential or logarithmic,
not quadratic.

Regardless, the same temperature decay schedule is always followed. That means
if the model update variance decreases like $\bigO{1/k^2}$ when the batch size
is increasing, the same schedule should be followed when the learning rate is
decayed. That implementation is shown with HSGD-2, which mirrors similar work
that decays the learning rate by the same factor the batch size would have
increased~\cite{smith2017,
adabatch}.\footnote{\href{https://github.com/NVlabs/AdaBatch/blob/e8d0de67c387ab1e9fcadab9713113f9b0fec728/adabatch\_cifar.py\#L278-L287}{https://github.com/NVlabs/AdaBatch/\ldots/adabatch\_cifar.py\#L278-L287}}
Therefore, in HSGD-2 the learning rate is decayed like $\bigO{1/k^2}$ after a
maximum batch size is reached even though it violates the conditions set forth
by~\citet{robbins1951}.

\begin{figure*}[t]
    \centering
    \begin{subfigure}[b]{0.30\textwidth}
        \centering
        \includegraphics[height=0.18\textheight]{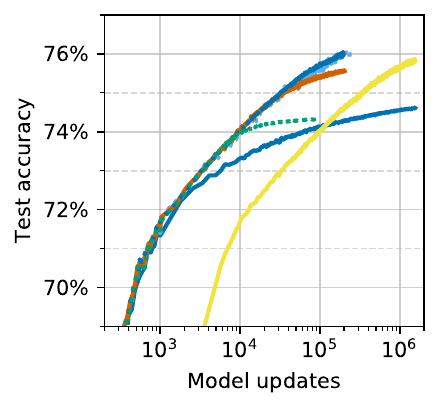}
        \caption{How test accuracy varies with the number of model updates.\\}
        \label{fig:padadamp-hsgd-test-updates}
    \end{subfigure}
    ~
    \begin{subfigure}[b]{0.30\textwidth}
        \centering
        \includegraphics[height=0.18\textheight]{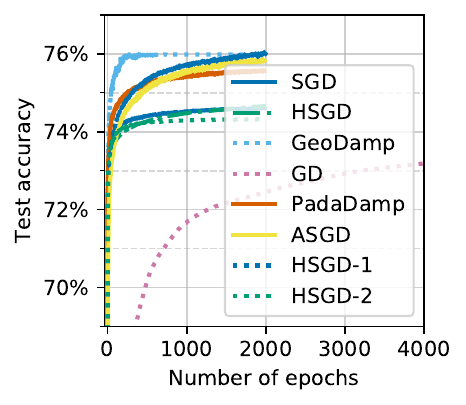}
        \caption{How test accuracy varies with the number of epochs. GD requires 32,100 epochs to reach 75\% accuracy.}
        \label{fig:padadamp-hsgd-train-epochs}
    \end{subfigure}
    ~
    \begin{subfigure}[b]{0.30\textwidth}
        \centering
        \includegraphics[height=0.18\textheight]{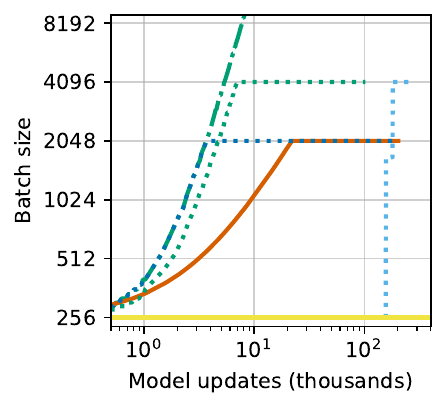}
        \caption{How the batch size varies with the number of model updates.\\}
        \label{fig:padadamp-hsgd-batch-size}
    \end{subfigure}
    \caption{%
        Various performance metrics for the experiment in
        Section~\ref{sec:padadamp} with two additional optimizers to adapt HSGD
        to maximum batch sizes. Gradient descent (GD) requires 32,100 epochs to
        reach 75\% accuracy; correspondingly, the x-axis in
        Figure~\ref{fig:padadamp-hsgd-train-epochs} is trimmed.
``HSGD-1'' and ``HSGD-2'' decay the learning rate like $\bigO{1/k}$ and
$\bigO{1/k^2}$ respectively after the maximum batch size is reached.
    }\label{fig:padadamp-hsgd}
\end{figure*}

We tuned HSGD-1 and HSGD-2 with the same method in \ref{app:padadamp-hyperopt}
with the batch size growth rate $m$ log-uniform for $m \in [10^{-3}, 10^{-1}]$.
All other parameters were fixed to be the final values, including the initial
batch size $B_0 = 256$, the initial learning rate $\gamma_0 = 0.9\cdot
10^{-3}$.  Then, the batch size $B_k = B_0 + \ceil*{m k^2}$. When $B_k >
B_{\max}$, the learning rate $\gamma_k = \gamma_0 B_{\max}/B_k$.

We initially ran HSGD-2 with maximum batch size $B_{\max} = 2048$ like the
other methods, but HSGD-2 didn't achieve high test accuracy with that maximum
batch size. We increased the maximum batch size to be $B_{\max} = 4096$ and got
the accuracy shown, significantly better.

Again, all optimizers have the same initialization and data ordering.

\subsection{CIFAR-10}\label{app:tune-cifar}\label{sec:cifar10}\label{app:cifar10}

These experiments mirror the experiments by Smith et al.~\cite{smith2017} and
L.  Smith~\cite{smith2018hyperparam}. GeoDamp rather significantly outperforms
\PadaDamp, which in turn outperforms SGD with geometrically decaying step
sizes. The experimental results are shown in Figure~\ref{fig:exp-cifar}.  In
both these experiments, all optimizers include Nestrov
momentum~\cite{nesterov2013a}.

The CIFAR-10 dataset has 50,000 training images and 10,000 images that fall
into 10 classes (e.g., ``bird'' or ``airplane''). All images are color and
$32\times 32$. The standard normalization is used to make the pixels zero mean
and unit variance in each
plane.\footnote{\href{https://github.com/kuangliu/pytorch-cifar/blob/882d877b8c816d85663a918015b9bacc07574fe2/main.py\#L34}{\texttt{kuangliu/pytorch-cifar/.../main.py\#L34}}}

Following the implementation of Wide-ResNet in Smith et al.~\cite{smith2017},
the ``16-4'' configuration of Wide-ResNet uses learning rate 0.1 and an initial
batch size of 128. We trained these models for 210 epochs. Every 60 epochs, the
batch size increases by a factor of 5 for GeoDamp. For SGD, every 60 epochs the
learning rate decays by a factor of 5.

In this, a slightly modified version of \PadaDamp~is used. This version of
\PadaDamp~is specifically designed to mirror the batch size increase shown in
Figure~\ref{fig:fashionmnist-batch-size}, the reason for including the decay
constant $\tau$. The default value provided is obtained from the experiment in
Section~\ref{sec:fmnist} and is not tuned in this section. Comparatively,
GeoDamp geometrically increases the batch size as a function of epochs.

\begin{algorithm}[H]
    \caption{\PadaDamp(batch size growth rate $m$, \AdaDamp~arguments)}
    \label{alg:padadamp2}
\begin{algorithmic}[1]
    % \Procedure{PadaDamp}{}
    \STATE\hspace{-1.5em}The same implementation as \AdaDamp,
     except line 5 is replaced with these lines:
    \STATE $\tilde{B}_k = B_0 + \ceil*{m\cdot k}$
    \STATE $B_k = \max\{B_0/4, \left(1 - e^{-k\cdot \tau}\right)\tilde{B}_k\}$
% \EndProcedure
\end{algorithmic}
\end{algorithm}

In our experiments, GeoDamp reaches testing accuracy that's about 2\% higher
than \PadaDamp's testing accuracy, and with the same number of model updates.
\PadaDamp~and GeoDamp LR reach similar testing accuracies after a given number
of epochs; however, \PadaDamp~requires fewer model updates to reach the same
testing accuracy.

\paragraph{Comparison with related work}
Our experiments do not reach the CIFAR-10 test set accuracy of about 94\% that
Smith et al. obtained~\cite[Fig.~3b]{smith2017}, though \PadaDamp~does
outperform the Wide-ResNet with 32 layers in the work by L.
Smith~\cite[Table~2]{smith2018hyperparam}, which obtains a CIFAR-10 testing
accuracy of between $88.7\% \pm 0.6$ after training for 200 epochs.

\begin{figure*}[t]
    \centering
    \begin{subfigure}[b]{0.3\textwidth}
        \centering
        \includegraphics[height=0.18\textheight]{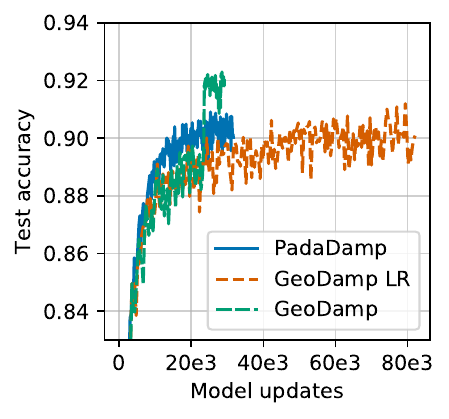}
        \caption{The number of model updates ($u$) vs. test accuracy.}
        \label{fig:cifar-test-updates}
    \end{subfigure}
    ~
    \begin{subfigure}[b]{0.3\textwidth}
        \centering
        \includegraphics[height=0.18\textheight]{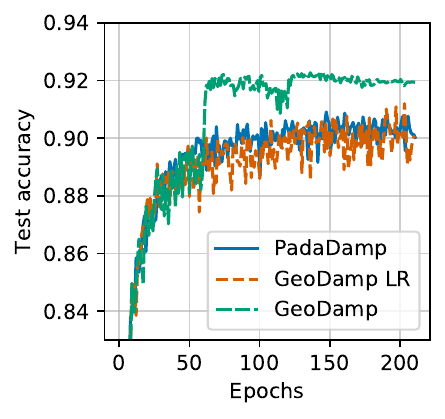}
        \caption{The number of epochs vs. test accuracy.}
        \label{fig:cifar-train-epochs}
    \end{subfigure}
    ~
    \begin{subfigure}[b]{0.3\textwidth}
        \centering
        \includegraphics[height=0.18\textheight]{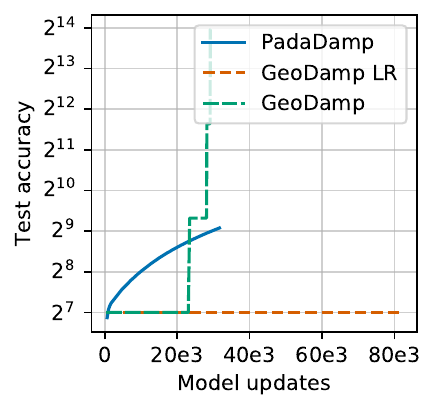}
        \caption{How the batch sizes changes with model updates.}
        \label{fig:cifar-batch-size}
    \end{subfigure}
    \caption{%
        Different performance metrics for \PadaDamp, GeoDamp and GeoDamp LR on the CIFAR-10 dataset. Details are in Section~\ref{sec:cifar10}.
    }\label{fig:exp-cifar}
\end{figure*}

\subsubsection{Hyperparameter optimization}

We followed previous work to allow easy comparison and avoid extensive
hyperparameter tuning. We still performed some basic tuning. Below, we'll describe the hyperparameter space then describe the tuning algorithm.

Unless otherwise mentioned, these hyperparameters were used:

\begin{itemize}
        \tightlist
    \item Learning rate: 0.1.
    \item Momentum: 0.9.
    \item Nestrov momentum: True.
    \item Initial batch size: 128
\end{itemize}

This mirrors the work of Smith et. al~\cite{smith2017}, so this completely
specifies the GeoDamp configuration.  For PadaDamp, we tuned the following
variables:

\begin{itemize}
        \tightlist
    \item Momentum, sampled uniformly between 0 and 1. (\textbf{tuned value}: approximately $0.87$. That gave motivation to choose a momentum value of 0.9 to mirror existing work).
    \item The relaxation time or ``dwell'' parameter: sampled uniformly from the list [1, 2, 5, 10, 20, 50, 100, 200, 500]. (\textbf{tuned value: 10}).
    \item Batch size growth rate: sampled log uniformly from the space between $10^{-4}$ and $10^{-1.5}$. (\textbf{tuned value: 0.013022})
    \item Maximum batch size: sampled uniformly from the list [128, 256, 512, 1024, 2048]. (\textbf{tuned value: 1024}. \PadaDamp~never obtained this
        maximum batch size.).
\end{itemize}

The hyperparameter optimization algorithm used is similar to median
elimination~\cite[Section 3.2.2]{golovin2017google} or successive
halving~\cite{karnin2013}:

\begin{enumerate}
        \tightlist
    \item Sample 200 hyperparameters. Run each for 20 epochs.
    \item Choose the top 60 models from (1). Run those models for 60 epochs.
    \item Choose the top 50 models from (2). Run those models for 180 epochs.
    \item Choose the top 10 models from (3). Run those models for 210 epochs,
        and average over 3 random seeds that determine the order in which examples are seen.
\end{enumerate}

Model initialization remained constant through all steps.  Steps (2) and (3)
defined ``top $N$'' as ``the $N$ models with the lowest loss.'' Step (4)
defined ``top 10'' as ``10 models with low loss and high accuracy.'' We chose
the tuned set of hyperparameters from one of the 10 models that had few model
updates and high validation accuracy. These 10 models all reached similar
average validation accuracies (within 1\%) but the number of model updates
varied significantly (by about a factor of $4$).

Steps (2), (3) and (4) used different validation sets. We only used the
provided test \emph{once} to create Figure~\ref{fig:exp-cifar}.
